# Supplementary material for: Stochastic lumping analysis for linear kinetics and its application to the fluctuation relations between hierarchical kinetic networks
Source: arXiv:1504.03092 source file (2015-04-13)
Supplement: Supplementary file 1 [file SI_17.pdf]

Supplementary Material for

# Stochastic lumping analysis for linear kinetics and its application to the fluctuation relations between hierarchical kinetic networks

De-Ming Deng and Cheng-Hung Chang

## Contents

S1 An example for lumping ........ 1
S2 Lumping chemical master equations ........ 1
S3 The TE condition on the stationary distributions ........ 7
S4 The indistinguishable $\boldsymbol{\Gamma}$ of intrinsic noises ........ 8

### S1. An example for lumping

**Example**: Let $A$ be a closed network with six states 1, … , 6 and $A'$ be another closed network with three states 1’, … , 3’.

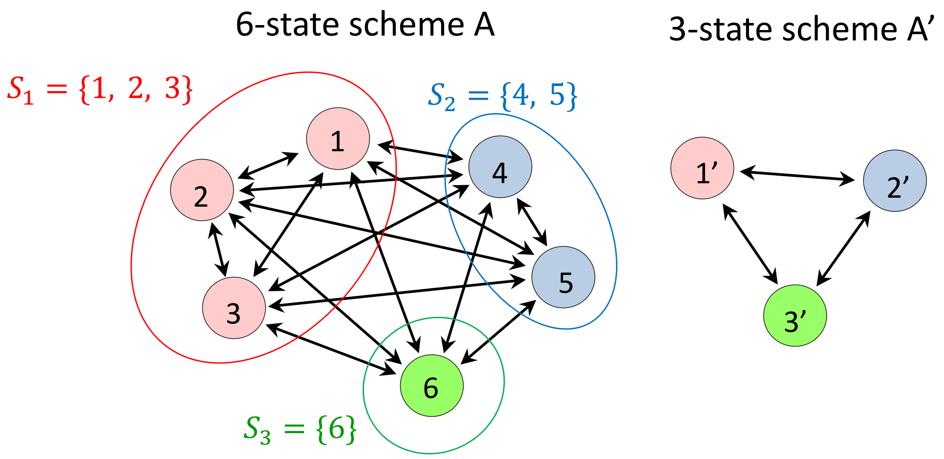


$A$ can be lumped into $A'$ by a $3 \times 6$ proper lumping matrix $\mathbf{U} = \begin{bmatrix} 1 & 1 & 1 & 0 & 0 & 0 \\ 0 & 0 & 0 & 1 & 1 & 0 \\ 0 & 0 & 0 & 0 & 0 & 1 \end{bmatrix}$.

This lumping process will group the six states of $A$ into three sets $S_1 = \{1,2,3\}$, $S_2 = \{4,5\}$, and $S_3 = \{6\}$ and merge the states in $S_1$ into state 1’ of $A'$, the states in $S_2$ into state 2’ of $A'$, and rename the state in $S_3$ as state 3’ of $A'$.

### S2. Lumping chemical master equations

The lumping matrix $\mathbf{U}$ associated lumping operator $\widehat{\mathbf{U}}$ defined in (8) will contract $\mathbf{P}$ into

$$\mathbf{P}' = \widehat{\mathbf{U}}\mathbf{P}, \tag{2.1}$$

whose $\widetilde{\mathbf{N}}'$-th component is

$$P'_{\widetilde{\mathbf{N}}'}(t) = \sum\nolimits_{\mathbf{U}\widetilde{\mathbf{N}}=\widetilde{\mathbf{N}}'} P_{\widetilde{\mathbf{N}}}(t) \equiv \sum_{\widetilde{\mathbf{N}}} P_{\widetilde{\mathbf{N}}}(t) \prod_{c=1}^{n'} \delta\left(\widetilde{N}'_c - \sum_{k\in S_c} \widetilde{N}_k\right). \qquad (2.2)$$

Here, $\sum_{\mathbf{U}\widetilde{\mathbf{N}}=\widetilde{\mathbf{N}}'}$ sums over all $\widetilde{\mathbf{N}}$ with $\widetilde{N}_1, \widetilde{N}_2, \ldots, \widetilde{N}_n \geq 0$, $\sum_{i=1}^{n} \widetilde{N}_i = N$, and $\mathbf{U}\widetilde{\mathbf{N}} = \widetilde{\mathbf{N}}'$. It is equivalent to the sum $\sum_{\widetilde{\mathbf{N}}}$ over all $\widetilde{\mathbf{N}}$ with $\widetilde{N}_1, \widetilde{N}_2, \ldots, \widetilde{N}_n \geq 0$ as well as $\sum_{i=1}^{n} \widetilde{N}_i = N$ and an extra Kronecker delta $\delta(\ldots)$ to select non-zero terms. These two sums are to merge all components of the vector equation (6) indexed by $\widetilde{\mathbf{N}}$ which can be lumped into the components $\widetilde{\mathbf{N}}'$ via $\mathbf{U}$. Thus, (2.2) is like the conventional expression, $f(x') = \int_{-\infty}^{\infty} f(x)\delta(x - x')dx$, of a delta function.

<u>**Example**</u>: The accessible $\widetilde{\mathbf{N}}$ which can be contracted by $\mathbf{U} = \begin{bmatrix} 1 & 1 & 0 \\ 0 & 0 & 1 \end{bmatrix}$ into $\widetilde{\mathbf{N}}' = \begin{bmatrix} 1 \\ 1 \end{bmatrix}$ are $\begin{bmatrix} 1 \\ 0 \\ 1 \end{bmatrix}$ and $\begin{bmatrix} 0 \\ 1 \\ 1 \end{bmatrix}$. Thus, $P'_{\widetilde{\mathbf{N}}'}(t) = P'_{[1,1]^T}(t) = P_{[1,0,1]^T}(t) + P_{[0,1,1]^T}(t)$.

<u>**Claim**</u>: The exact lumpability in the RE implies the exact lumpability in the CME and vice versa.

<u>Proof</u>:

For simplicity, we drop the time $t$ in $P_{\widetilde{\mathbf{N}}}(t)$ and $P'_{\widetilde{\mathbf{N}}'}(t)$ and abbreviate $\delta(X' - X)$ in (2.2) as $\delta_X^{X'}$. Furthermore, we will replace $\sum_{\mathbf{U}\widetilde{\mathbf{N}}=\widetilde{\mathbf{N}}'}$ and $\sum_{\widetilde{\mathbf{N}}}$ in (2.2) by $\sum^*_{\mathbf{U}\widetilde{\mathbf{N}}=\widetilde{\mathbf{N}}'}$ and $\sum^*_{\widetilde{\mathbf{N}}}$ , where the asterisk means the sums are over "all integers" $\widetilde{N}_1, \widetilde{N}_2, \ldots, \widetilde{N}_n$ and does not exclude the $P_{\widetilde{\mathbf{N}}}(t)$ of negative $\widetilde{N}_i$. This will considerably simplify the proof and the original boundary condition that $P_{\widetilde{\mathbf{N}}}(t) \equiv 0$ for any $\widetilde{N}_i < 0$ is only a special case.

For the forward direction of the claim, we operate $\sum^*_{\mathbf{U}\widetilde{\mathbf{N}}=\widetilde{\mathbf{N}}'}$ on both sides of (6) in the main text,

$$\frac{d\sum^*_{\mathbf{U}\widetilde{\mathbf{N}}=\widetilde{\mathbf{N}}'} P_{\widetilde{\mathbf{N}}}}{dt} = \sum_{\mathbf{U}\widetilde{\mathbf{N}}=\widetilde{\mathbf{N}}'}^{*} \sum_{i,j=1}^{n} k_{ij} \left[(\widetilde{N}_i + 1)P_{\widetilde{\mathbf{N}}-\boldsymbol{\omega}_{ij}} - \widetilde{N}_i P_{\widetilde{\mathbf{N}}}\right]$$

$$= \sum_{\mathbf{U}\widetilde{\mathbf{N}}=\widetilde{\mathbf{N}}'}^{*} \sum_{a=1}^{n'} \sum_{i\in S_a} \sum_{j\in S_a} k_{ij}(\widetilde{N}_i + 1)P_{\widetilde{\mathbf{N}}-\boldsymbol{\omega}_{ij}} - \sum_{\mathbf{U}\widetilde{\mathbf{N}}=\widetilde{\mathbf{N}}'}^{*} \sum_{a=1}^{n'} \sum_{i\in S_a} \sum_{j\in S_a} k_{ij}\widetilde{N}_i P_{\widetilde{\mathbf{N}}}$$

$$+ \sum_{\mathbf{U}\widetilde{\mathbf{N}}=\widetilde{\mathbf{N}}'}^{*} \sum_{a=1}^{n'} \sum_{b\neq a}^{n'} \sum_{i\in S_a} \sum_{j\in S_b} k_{ij}(\widetilde{N}_i + 1)P_{\widetilde{\mathbf{N}}-\boldsymbol{\omega}_{ij}} - \sum_{\mathbf{U}\widetilde{\mathbf{N}}=\widetilde{\mathbf{N}}'}^{*} \sum_{a=1}^{n'} \sum_{b\neq a}^{n'} \sum_{i\in S_a} \sum_{j\in S_b} k_{ij}\widetilde{N}_i P_{\widetilde{\mathbf{N}}}. \qquad (2.3)$$

Let us denote the four terms in (2.3) as $I_i$ with $i = 1, \dots, 4$. In the first term,

$$I_1 = \sum_{\mathbf{U}\widetilde{\mathbf{N}}=\widetilde{\mathbf{N}}'}^{*} \sum_{a=1}^{n'} \sum_{i\in S_a} \sum_{j\in S_a} k_{ij}(\widetilde{N}_i + 1) P_{\widetilde{\mathbf{N}}-\boldsymbol{\omega}_{ij}}. \quad (2.4)$$

If we replace $\widetilde{\mathbf{N}}$ by $\widetilde{\mathbf{N}} + \boldsymbol{\omega}_{ij}$, $\widetilde{N}_i$ and $\widetilde{N}_j$ will be replaced by $\widetilde{N}_i - 1$ and $\widetilde{N}_j + 1$, respectively. Furthermore, $\mathbf{U}\widetilde{\mathbf{N}} = \widetilde{\mathbf{N}}'$ will be replaced by $\mathbf{U}(\widetilde{\mathbf{N}} + \boldsymbol{\omega}_{ij}) = \widetilde{\mathbf{N}}'$, which is equal to $\mathbf{U}\widetilde{\mathbf{N}} = \widetilde{\mathbf{N}}'$ because $i$ and $j$ in (2.4) belong to the same set $S_a$ and then $\mathbf{U}\boldsymbol{\omega}_{ij} = 0$. Thus,

$$I_1 = \sum_{\mathbf{U}\widetilde{\mathbf{N}}=\widetilde{\mathbf{N}}'}^{*} \sum_{a=1}^{n'} \sum_{i\in S_a} \sum_{j\in S_a} k_{ij} \widetilde{N}_i P_{\widetilde{\mathbf{N}}} = -I_2$$

and subsequently $I_1 + I_2 = 0$. The third term is

$$I_3 = \sum_{\mathbf{U}\widetilde{\mathbf{N}}=\widetilde{\mathbf{N}}'}^{*} \sum_{a=1}^{n'} \sum_{b\neq a}^{n'} \sum_{i\in S_a} \sum_{j\in S_b} k_{ij}(\widetilde{N}_i + 1) P_{\widetilde{\mathbf{N}}-\boldsymbol{\omega}_{ij}}$$

$$\underbrace{=}_{(2.2)} \sum_{\widetilde{\mathbf{N}}}^{*} \sum_{a=1}^{n'} \sum_{b\neq a}^{n'} \sum_{i\in S_a} \sum_{j\in S_b} k_{ij}(\widetilde{N}_i + 1) P_{\widetilde{\mathbf{N}}-\boldsymbol{\omega}_{ij}} \prod_{c=1}^{n'} \delta_{\sum_{k\in S_c} \widetilde{N}_k}^{\widetilde{N}'_c}$$

$$= \sum_{\widetilde{\mathbf{N}}}^{*} \sum_{a=1}^{n'} \sum_{b\neq a}^{n'} \sum_{i\in S_a} \sum_{j\in S_b} k_{ij}(\widetilde{N}_i + 1) P_{[\widetilde{N}_1, \dots, \widetilde{N}_i+1, \dots, \widetilde{N}_j-1, \dots, \widetilde{N}_n]^T}$$

$$\times \delta_{(\widetilde{N}_i+1)+\sum_{k\in S_a, k\neq i} \widetilde{N}_k}^{\widetilde{N}'_a+1} \delta_{(\widetilde{N}_j-1)+\sum_{k\in S_b, k\neq j} \widetilde{N}_k}^{\widetilde{N}'_b-1} \prod_{c\neq a,b}^{n'} \delta_{\sum_{k\in S_c} \widetilde{N}_k}^{\widetilde{N}'_c}, \quad (2.5)$$

where $\sum_{b\neq a}^{n'}$ runs over all $b = 1, \dots, n'$ with $b \neq a$ and $\prod_{c\neq a,b}^{n'}$ extends over all $c = 1, \dots, n'$ with $c \neq a$ and $b$. Using the KE condition (5), $\sum_{j\in S_b} k_{ij} = k'_{ab}$, and replacing $\widetilde{N}_i + 1$ by $\widetilde{N}_i$ and $\widetilde{N}_j - 1$ by $\widetilde{N}_j$, (2.5) becomes

$$I_3 = \sum_{\widetilde{\mathbf{N}}}^{*} \sum_{a=1}^{n'} \sum_{b\neq a}^{n'} \sum_{i\in S_a} k'_{ab} \widetilde{N}_i P_{\widetilde{\mathbf{N}}} \delta_{\sum_{k\in S_a} \widetilde{N}_k}^{\widetilde{N}'_a+1} \delta_{\sum_{k\in S_b} \widetilde{N}_k}^{\widetilde{N}'_b-1} \prod_{c\neq a,b}^{n'} \delta_{\sum_{k\in S_c} \widetilde{N}_k}^{\widetilde{N}'_c}$$

$$= \sum_{a=1}^{n'} \sum_{b\neq a}^{n'} k'_{ab} \sum_{\widetilde{\mathbf{N}}}^{*} \sum_{i\in S_a} \widetilde{N}_i P_{\widetilde{\mathbf{N}}} \delta_{\sum_{k\in S_a} \widetilde{N}_k}^{\widetilde{N}'_a+1} \delta_{\sum_{k\in S_b} \widetilde{N}_k}^{\widetilde{N}'_b-1} \prod_{c\neq a,b}^{n'} \delta_{\sum_{k\in S_c} \widetilde{N}_k}^{\widetilde{N}'_c}. \quad (2.6)$$

Therein, $\sum_{\widetilde{\mathbf{N}}}^{*}$ and $\sum_{a=1}^{n'} \sum_{b\neq a}^{n'}$ have been exchanged since $\sum_{\widetilde{\mathbf{N}}}^{*}$ and $\sum_{i,j}^{n} = \sum_{a=1}^{n'} \sum_{b\neq a}^{n'} \sum_{i\in S_a} \sum_{j\in S_b}$, and subsequently $\sum_{\widetilde{\mathbf{N}}}^{*}$ and $\sum_{a=1}^{n'} \sum_{b\neq a}^{n'}$, are independent sums, because $\sum_{i,j}^{n}$ runs over the index $i$ of $\widetilde{N}_i$, while $\sum_{\widetilde{\mathbf{N}}}^{*}$ sums over the accessible values of $\widetilde{N}_i$. The Kronecker delta $\delta_{\sum_{k\in S_a} \widetilde{N}_k}^{\widetilde{N}'_a+1}$ in (2.6) not only tells us that the sum $\sum_{i\in S_a} \widetilde{N}_i$ before $P_{\widetilde{\mathbf{N}}}$

must be equal to $\widetilde{N}'_a + 1$ but also which $P_{\widetilde{\mathbf{N}}}$ will appear in the sum $\sum^*_{\widetilde{\mathbf{N}}}$ . Under definition (2.2) with $\sum_{\widetilde{\mathbf{N}}}$ replaced by $\sum^*_{\widetilde{\mathbf{N}}}$ , one has

$$\sum_{\widetilde{\mathbf{N}}}^{*} P_{\widetilde{\mathbf{N}}}\, \delta^{\widetilde{N}'_a+1}_{\sum_{k\in S_a}\widetilde{N}_k}\, \delta^{\widetilde{N}'_b-1}_{\sum_{k\in S_b}\widetilde{N}_k} \prod_{c\neq a,b}^{n'} \delta^{\widetilde{N}'_c}_{\sum_{k\in S_c}\widetilde{N}_k} = P'_{\left[\widetilde{N}'_1,\dots,\widetilde{N}'_a+1,\dots,\widetilde{N}'_b-1,\dots\widetilde{N}'_{n'}\right]^T}. \tag{2.7}$$

Inserting (2.7) into (2.6), it yields

$$I_3 = \sum_{a=1}^{n'}\sum_{b\neq a}^{n'} k'_{ab}\left(\widetilde{N}'_a + 1\right) P'_{\left[\widetilde{N}'_1,\dots,\widetilde{N}'_a+1,\dots,\widetilde{N}'_b-1,\dots\widetilde{N}'_{n'}\right]^T} = \sum_{a,b=1}^{n'} k'_{ab}\left(\widetilde{N}'_a + 1\right) P'_{\widetilde{\mathbf{N}}'-\boldsymbol{\omega}'_{ab}}, \tag{2.8}$$

where $k'_{aa} \equiv 0$ as defined after (3). With the same argument, the fourth term in (2.3) is

$$I_4 = -\sum_{a,b=1}^{n'} k'_{ab} N'_a P'_{\widetilde{\mathbf{N}}'}. \tag{2.9}$$

Substituting $I_1 \sim I_4$ into (2.3), we obtain (9). It is nothing but the CME of $A'$, whose rate constants are related to those of $A$ by the KE condition (5). Thus, $\mathbf{P}' = \widehat{\mathbf{U}}\mathbf{P}$ obey the CME of $A'$.

Conversely, suppose $\mathbf{P}$ and $\mathbf{P}'$ of the CMEs of $A$ and $A'$ are related by $\widehat{\mathbf{U}}\mathbf{P} = \mathbf{P}'$. The $\widehat{\mathbf{U}}$ associated $\mathbf{U}$ will partition the states in $A$ into $n'$ sets $S_c$, with $\mathrm{c} = 1, 2, \dots, n'$ and give the identity

$$\sum\nolimits^*_{\widetilde{\mathbf{N}}'} \prod_{c=1}^{n'} \delta^{\widetilde{N}'_c}_{\sum_{k\in S_c}\widetilde{N}_k} = 1. \tag{2.10}$$

As an example, for $\mathbf{U} = \begin{bmatrix} 1 & 1 & 0 \\ 0 & 0 & 1 \end{bmatrix}$ and $\widetilde{\mathbf{N}} = [1, 3, 2]^T$, (2.10) means $\sum^*_{\widetilde{\mathbf{N}}'} \delta\left(\widetilde{N}'_1 - \widetilde{N}_1 - \widetilde{N}_2\right)\delta\left(\widetilde{N}'_2 - \widetilde{N}_3\right) = \sum^*_{\widetilde{\mathbf{N}}'} \delta\left(\widetilde{N}'_1 - 4\right)\delta\left(\widetilde{N}'_2 - 2\right) = 1$. It is like $\int \delta(x - x')\, dx = 1$ for a normal delta function. Using (2.10) and (2.2), the $a$-th component of the merged mean will be

$$[\mathbf{UN}]_a = \sum_{i\in S_a} N_i = \sum_{i\in S_a}\sum_{\widetilde{\mathbf{N}}}^{*} \widetilde{N}_i P_{\widetilde{\mathbf{N}}} \underbrace{=}_{(2.10)} \sum_{\widetilde{\mathbf{N}}}^{*}\left(\sum_{i\in S_a}\widetilde{N}_i\right) P_{\widetilde{\mathbf{N}}} \sum_{\widetilde{\mathbf{N}}'}^{*}\prod_{c=1}^{n'} \delta^{\widetilde{N}'_c}_{\sum_{k\in S_c}\widetilde{N}_k}$$

$$= \sum_{\widetilde{\mathbf{N}}'}^{*}\sum_{\widetilde{\mathbf{N}}}^{*}\left(\sum_{i\in S_a}\widetilde{N}_i\right) P_{\widetilde{\mathbf{N}}} \prod_{c=1}^{n'} \delta^{\widetilde{N}'_c}_{\sum_{k\in S_c}\widetilde{N}_k} \underbrace{=}_{(2.2)} \sum_{\widetilde{\mathbf{N}}'}^{*} \widetilde{N}'_a P'_{\widetilde{\mathbf{N}}'} = [\mathbf{N}']_a. \tag{2.11}$$

Thus, if the REs and CMEs of $A$ and $A'$ are given, then $\widehat{\mathbf{U}}\mathbf{P} = \mathbf{P}'$ implies $\mathbf{UN} = \mathbf{N}'$.

Following the same strategy, the extension to other moments is straightforward. The "$\boldsymbol{m}$-th" moment of the variable $\mathbf{U}\widetilde{\mathbf{N}}$, with the vector $\boldsymbol{m} = [m_1, m_2, \dots m_{n'}]$, is

$$\langle\prod_{b=1}^{n'}\left(\sum_{j\in S_b}\widetilde{N}_j\right)^{m_b}\rangle \equiv \sum_{\widetilde{\mathbf{N}}}^{*}\prod_{b=1}^{n'}\left(\sum_{j\in S_b}\widetilde{N}_j\right)^{m_b} P_{\widetilde{\mathbf{N}}}. \tag{2.12}$$

As an example, if $m_b$ is a Kronecker delta $\delta_{ba}$, (2.12) will represent the $a$-th mean value of $\mathbf{U}\widetilde{\mathbf{N}}$, i.e., $[\mathbf{UN}]_a = \sum_{\widetilde{\mathbf{N}}}^{*}\sum_{i\in S_a}\widetilde{N}_i P_{\widetilde{\mathbf{N}}}$. In analogy to (2.11), one has

$$\begin{aligned}\langle\prod_{b=1}^{n'}\left(\sum_{j\in S_b}\widetilde{N}_j\right)^{m_b}\rangle &= \sum_{\widetilde{\mathbf{N}}}^{*}\prod_{b=1}^{n'}\left(\sum_{j\in S_b}\widetilde{N}_j\right)^{m_b} P_{\widetilde{\mathbf{N}}} \underbrace{=}_{(2.10)} \sum_{\widetilde{\mathbf{N}}}\prod_{b=1}^{n'}\left(\sum_{j\in S_b}\widetilde{N}_j\right)^{m_b} P_{\widetilde{\mathbf{N}}}\sum_{\widetilde{\mathbf{N}}'}^{*}\prod_{c=1}^{n'}\delta_{\sum_{k\in S_c}\widetilde{N}_k}^{\widetilde{N}'_c}\\ &= \sum_{\widetilde{\mathbf{N}}'}^{*}\sum_{\widetilde{\mathbf{N}}}^{*}P_{\widetilde{\mathbf{N}}}\prod_{b=1}^{n'}\left(\sum_{j\in S_b}\widetilde{N}_j\right)^{m_b}\delta_{\sum_{j\in S_b}\widetilde{N}_j}^{\widetilde{N}'_b} \underbrace{=}_{(2.2)} \sum_{\widetilde{\mathbf{N}}'}^{*}\prod_{b=1}^{n'}\left(\widetilde{N}'_b\right)^{m_b}P'_{\widetilde{\mathbf{N}}'}\\ &= \langle\prod_{b=1}^{n'}\left(\widetilde{N}'_b\right)^{m_b}\rangle,\end{aligned} \tag{2.13}$$

which implies the identity between the $\boldsymbol{m}$-th moments of $\mathbf{U}\widetilde{\mathbf{N}}$ and $\widetilde{\mathbf{N}}'$. As a special case, substituting $m_b = \delta_{ba}$ into (2.13) gives the first moment relation

$$[\mathbf{UN}]_a = \sum_{i\in S_a}\langle\widetilde{N}_i\rangle = \langle\sum_{i\in S_a}\widetilde{N}_i\rangle \underbrace{=}_{(2.13)} \langle\widetilde{N}'_a\rangle = [\mathbf{N}']_a. \tag{2.14}$$

The relation of second moments (11) in the main text is another example of (2.13). Notably, (2.13) can also be derived by the characteristic function of $\widehat{\mathbf{U}}\mathbf{P} = \mathbf{P}'$. ■

**Example:** Under the boundary condition that $P_{\widetilde{\mathbf{N}}} = 0$ for any $\widetilde{N}_i < 0$, (2.3) becomes

$$\frac{d\sum_{\mathbf{U}\widetilde{\mathbf{N}}=\widetilde{\mathbf{N}}'}P_{\widetilde{\mathbf{N}}}}{dt} = \sum_{\mathbf{U}\widetilde{\mathbf{N}}=\widetilde{\mathbf{N}}'}\sum_{i,j=1}^{n}k_{ij}\left[\left(\widetilde{N}_i+1\right)P_{\widetilde{\mathbf{N}}-\boldsymbol{\omega}_{ij}} - \widetilde{N}_iP_{\widetilde{\mathbf{N}}}\right]. \tag{2.15}$$

For $\widetilde{\mathbf{N}} \equiv \begin{bmatrix}\widetilde{N}_1\\ \widetilde{N}_2\\ \widetilde{N}_3\end{bmatrix}$ and $\mathbf{U} = \begin{bmatrix}1 & 1 & 0\\ 0 & 0 & 1\end{bmatrix}$, consider the transition $\boldsymbol{\omega}_{ij} = \boldsymbol{\omega}_{13}$ and denote the probability $P_{\widetilde{\mathbf{N}}} = P_{[\widetilde{N}_1,\widetilde{N}_2,\widetilde{N}_3]^T}$ as $\begin{pmatrix}\widetilde{N}_1 & & \widetilde{N}_2\\ & \widetilde{N}_3 & \end{pmatrix}$, the rate of inflow from $\widetilde{\mathbf{N}} - \boldsymbol{\omega}_{13}$ into $\widetilde{\mathbf{N}}$ as

$$\begin{bmatrix}\widetilde{N}_1+1 & & \widetilde{N}_2\\ & \searrow & \\ & \widetilde{N}_3-1 & \end{bmatrix} \equiv k_{13}\left(\widetilde{N}_1+1\right)P_{\widetilde{\mathbf{N}}-\boldsymbol{\omega}_{13}} = k_{13}\left(\widetilde{N}_1+1\right)\begin{pmatrix}\widetilde{N}_1+1 & & \widetilde{N}_2\\ & \widetilde{N}_3-1 & \end{pmatrix},$$

and the rate of outflow out of $\widetilde{\mathbf{N}}$ into $\widetilde{\mathbf{N}} + \boldsymbol{\omega}_{13}$ as

$$\begin{bmatrix}\widetilde{N}_1 & & \widetilde{N}_2\\ & \searrow & \\ & \widetilde{N}_3 & \end{bmatrix} \equiv k_{13}\widetilde{N}_1P_{\widetilde{\mathbf{N}}} = k_{13}\widetilde{N}_1\begin{pmatrix}\widetilde{N}_1 & & \widetilde{N}_2\\ & \widetilde{N}_3 & \end{pmatrix},$$

where the arrow indicates the direction of transition from state $i=1$ to state $j=3$. For $\widetilde{\mathbf{N}}'=\begin{bmatrix}\widetilde{N}_1+\widetilde{N}_2\\ \widetilde{N}_3\end{bmatrix}=\begin{bmatrix}2\\2\end{bmatrix}$, the non-zero $\frac{d\sum_{\mathbf{U}\widetilde{\mathbf{N}}=\widetilde{\mathbf{N}}'}P_{\widetilde{\mathbf{N}}}}{dt}$ in (2.15) are

$$\frac{d}{dt}\begin{pmatrix}0 & & 2\\ & 2 & \end{pmatrix}=\cdots+\begin{bmatrix}-1\leftarrow 3\\ 2\end{bmatrix}+\begin{bmatrix}1\rightarrow 1\\ 2\end{bmatrix}+\begin{bmatrix}1 & & 2\\ & \searrow & \\ & 1 & \end{bmatrix}+\begin{bmatrix}0 & & 3\\ & \swarrow & \\ & 1 & \end{bmatrix}+\begin{bmatrix}-1 & & 2\\ & \nwarrow & \\ & 3 & \end{bmatrix}+\begin{bmatrix}0 & & 1\\ & \nearrow & \\ & 3 & \end{bmatrix}+\cdots$$
$$\cdots-\begin{bmatrix}0\leftarrow 2\\ 2\end{bmatrix}-\begin{bmatrix}0\rightarrow 2\\ 2\end{bmatrix}-\begin{bmatrix}0 & & 2\\ & \searrow & \\ & 2 & \end{bmatrix}-\begin{bmatrix}0 & & 2\\ & \swarrow & \\ & 2 & \end{bmatrix}-\begin{bmatrix}0 & & 2\\ & \nwarrow & \\ & 2 & \end{bmatrix}-\begin{bmatrix}0 & & 2\\ & \nearrow & \\ & 2 & \end{bmatrix}-\cdots$$
$$\frac{d}{dt}\begin{pmatrix}1 & & 1\\ & 2 & \end{pmatrix}=\cdots+\begin{bmatrix}0\leftarrow 2\\ 2\end{bmatrix}+\begin{bmatrix}2\rightarrow 0\\ 2\end{bmatrix}+\begin{bmatrix}2 & & 1\\ & \searrow & \\ & 1 & \end{bmatrix}+\begin{bmatrix}1 & & 2\\ & \swarrow & \\ & 1 & \end{bmatrix}+\begin{bmatrix}0 & & 1\\ & \nwarrow & \\ & 3 & \end{bmatrix}+\begin{bmatrix}1 & & 0\\ & \nearrow & \\ & 3 & \end{bmatrix}+\cdots$$
$$\cdots-\begin{bmatrix}1\leftarrow 1\\ 2\end{bmatrix}-\begin{bmatrix}1\rightarrow 1\\ 2\end{bmatrix}-\begin{bmatrix}1 & & 1\\ & \searrow & \\ & 2 & \end{bmatrix}-\begin{bmatrix}1 & & 1\\ & \swarrow & \\ & 2 & \end{bmatrix}-\begin{bmatrix}1 & & 1\\ & \nwarrow & \\ & 2 & \end{bmatrix}-\begin{bmatrix}1 & & 1\\ & \nearrow & \\ & 2 & \end{bmatrix}-\cdots$$
$$\frac{d}{dt}\begin{pmatrix}2 & & 0\\ & 2 & \end{pmatrix}=\cdots+\begin{bmatrix}1\leftarrow 1\\ 2\end{bmatrix}+\begin{bmatrix}3\rightarrow -1\\ 2\end{bmatrix}+\begin{bmatrix}3 & & 0\\ & \searrow & \\ & 1 & \end{bmatrix}+\begin{bmatrix}2 & & 1\\ & \swarrow & \\ & 1 & \end{bmatrix}+\begin{bmatrix}1 & & 0\\ & \nwarrow & \\ & 3 & \end{bmatrix}+\begin{bmatrix}2 & & -1\\ & \nearrow & \\ & 3 & \end{bmatrix}+\cdots$$
$$\cdots-\begin{bmatrix}2\leftarrow 0\\ 2\end{bmatrix}-\begin{bmatrix}2\rightarrow 0\\ 2\end{bmatrix}-\begin{bmatrix}2 & & 0\\ & \searrow & \\ & 2 & \end{bmatrix}-\begin{bmatrix}2 & & 0\\ & \swarrow & \\ & 2 & \end{bmatrix}-\begin{bmatrix}2 & & 0\\ & \nwarrow & \\ & 2 & \end{bmatrix}-\begin{bmatrix}2 & & 0\\ & \nearrow & \\ & 2 & \end{bmatrix}-\cdots.$$

From that it follows

$$I_1=\begin{bmatrix}1\rightarrow 1\\ 2\end{bmatrix}+\begin{bmatrix}0\leftarrow 2\\ 2\end{bmatrix}+\begin{bmatrix}2\rightarrow 0\\ 2\end{bmatrix}+\begin{bmatrix}1\leftarrow 1\\ 2\end{bmatrix}+\underbrace{\begin{bmatrix}-1\leftarrow 3\\ 2\end{bmatrix}}_{=0}+\underbrace{\begin{bmatrix}3\rightarrow -1\\ 2\end{bmatrix}}_{=0}$$
$$I_2=-\begin{bmatrix}0\leftarrow 2\\ 2\end{bmatrix}-\begin{bmatrix}1\leftarrow 1\\ 2\end{bmatrix}-\begin{bmatrix}1\rightarrow 1\\ 2\end{bmatrix}-\begin{bmatrix}2\rightarrow 0\\ 2\end{bmatrix}-\underbrace{\begin{bmatrix}0\rightarrow 2\\ 2\end{bmatrix}}_{=0}-\underbrace{\begin{bmatrix}2\leftarrow 0\\ 2\end{bmatrix}}_{=0}$$

and $I_1+I_2=0$. Furthermore,

$$I_3=\begin{bmatrix}1 & & 2\\ & \searrow & \\ & 1 & \end{bmatrix}+\begin{bmatrix}2 & & 1\\ & \searrow & \\ & 1 & \end{bmatrix}+\begin{bmatrix}3 & & 0\\ & \searrow & \\ & 1 & \end{bmatrix}+\begin{bmatrix}0 & & 1\\ & \nwarrow & \\ & 3 & \end{bmatrix}+\begin{bmatrix}1 & & 0\\ & \nwarrow & \\ & 3 & \end{bmatrix}+\underbrace{\begin{bmatrix}-1 & & 2\\ & \nwarrow & \\ & 3 & \end{bmatrix}}_{=0}$$
$$+\begin{bmatrix}0 & & 3\\ & \swarrow & \\ & 1 & \end{bmatrix}+\begin{bmatrix}1 & & 2\\ & \swarrow & \\ & 1 & \end{bmatrix}+\begin{bmatrix}2 & & 1\\ & \swarrow & \\ & 1 & \end{bmatrix}+\begin{bmatrix}0 & & 1\\ & \nearrow & \\ & 3 & \end{bmatrix}+\begin{bmatrix}1 & & 0\\ & \nearrow & \\ & 3 & \end{bmatrix}+\underbrace{\begin{bmatrix}2 & & -1\\ & \nearrow & \\ & 3 & \end{bmatrix}}_{=0}$$
$$=k_{13}\left[1\begin{pmatrix}1 & & 2\\ & 1 & \end{pmatrix}+2\begin{pmatrix}2 & & 1\\ & 1 & \end{pmatrix}+3\begin{pmatrix}3 & & 0\\ & 1 & \end{pmatrix}\right]+k_{31}\left[3\begin{pmatrix}0 & & 1\\ & 3 & \end{pmatrix}+3\begin{pmatrix}1 & & 0\\ & 3 & \end{pmatrix}\right]$$
$$+k_{23}\left[3\begin{pmatrix}0 & & 3\\ & 1 & \end{pmatrix}+2\begin{pmatrix}1 & & 2\\ & 1 & \end{pmatrix}+1\begin{pmatrix}2 & & 1\\ & 1 & \end{pmatrix}\right]+k_{32}\left[3\begin{pmatrix}0 & & 1\\ & 3 & \end{pmatrix}+3\begin{pmatrix}1 & & 0\\ & 3 & \end{pmatrix}\right].$$

Under the KE condition, $k_{13}=k_{23}=k'_{12}$ and $k_{31}+k_{32}=k'_{21}$, it yields

$$I_3=k'_{12}\left[1\begin{pmatrix}1 & & 2\\ & 1 & \end{pmatrix}+2\begin{pmatrix}2 & & 1\\ & 1 & \end{pmatrix}+3\begin{pmatrix}3 & & 0\\ & 1 & \end{pmatrix}+3\begin{pmatrix}0 & & 3\\ & 1 & \end{pmatrix}+2\begin{pmatrix}1 & & 2\\ & 1 & \end{pmatrix}+1\begin{pmatrix}2 & & 1\\ & 1 & \end{pmatrix}\right]$$
$$+k'_{21}\left[3\begin{pmatrix}0 & & 1\\ & 3 & \end{pmatrix}+3\begin{pmatrix}1 & & 0\\ & 3 & \end{pmatrix}\right]$$
$$=3k'_{12}\left[\begin{pmatrix}1 & & 2\\ & 1 & \end{pmatrix}+\begin{pmatrix}2 & & 1\\ & 1 & \end{pmatrix}+\begin{pmatrix}3 & & 0\\ & 1 & \end{pmatrix}+\begin{pmatrix}0 & & 3\\ & 1 & \end{pmatrix}\right]+3k'_{21}\left[\begin{pmatrix}0 & & 1\\ & 3 & \end{pmatrix}+\begin{pmatrix}1 & & 0\\ & 3 & \end{pmatrix}\right]$$

$$= 3k'_{12}P'\left(\begin{bmatrix}3\\1\end{bmatrix}\right) + 3k'_{21}P'\left(\begin{bmatrix}1\\3\end{bmatrix}\right)$$

$$= k'_{12}(2+1)P'\left(\begin{bmatrix}2\\2\end{bmatrix} - \begin{bmatrix}-1\\1\end{bmatrix}\right) + k'_{21}(2+1)P'\left(\begin{bmatrix}2\\2\end{bmatrix} - \begin{bmatrix}1\\-1\end{bmatrix}\right)$$

$$= \sum_{a,b=1}^{2} k'_{ab}\left(\widetilde{N}'_a + 1\right)P'_{\widetilde{\mathbf{N}}'-\boldsymbol{\omega}'_{ab}}.$$

**S3. The TE condition on the stationary distributions**

**<u>Claim</u>:** The TE condition, $\mathbf{N}'^{s} = \mathbf{U}\mathbf{N}^{s}$, holds if and only if $\mathbf{P}'^{s} = \widehat{\mathbf{U}}\mathbf{P}^{s}$.

<u>Proof</u>:

To see $\mathbf{N}'^{s} = \mathbf{U}\mathbf{N}^{s}$ implies $\mathbf{P}'^{s} = \widehat{\mathbf{U}}\mathbf{P}^{s}$, let us rewrite $P^{s}_{\widetilde{\mathbf{N}}}$ in (12) as

$$P^{s}_{\widetilde{\mathbf{N}}} = \frac{N!}{\prod_{i=1}^{n}\widetilde{N}_i!}\prod_{j=1}^{n}\left(\frac{N_j^s}{N}\right)^{\widetilde{N}_j} = \frac{N!}{N^N}\prod_{i=1}^{n}\frac{N_i^{s\,\widetilde{N}_i}}{\widetilde{N}_i!} = \frac{N!}{N^N}\prod_{a=1}^{n'}\prod_{i\in S_a}\frac{N_i^{s\,\widetilde{N}_i}}{\widetilde{N}_i!}$$

$$= \frac{N!}{N^N}\prod_{a=1}^{n'}\left(\frac{N_a'^{s\,\widetilde{N}'_a}}{\widetilde{N}'_a!}\frac{\widetilde{N}'_a!}{N_a'^{s\,\widetilde{N}'_a}}\prod_{i\in S_a}\frac{N_i^{s\,\widetilde{N}_i}}{\widetilde{N}_i!}\right) = \left[\frac{N!}{\prod_{a=1}^{n'}\widetilde{N}'_a!}\prod_{b=1}^{n'}\left(\frac{N_b'^{s}}{N}\right)^{\widetilde{N}'_b}\right]\prod_{c=1}^{n'}\left(\frac{\widetilde{N}'_c!}{N_c'^{s\,\widetilde{N}'_c}}\prod_{i\in S_c}\frac{N_i^{s\,\widetilde{N}_i}}{\widetilde{N}_i!}\right). \qquad (3.1)$$

Thus, the $\widetilde{\mathbf{N}}'$-th component of $\mathbf{P}'^{s}$ is

$$\sum_{\mathbf{U}\widetilde{\mathbf{N}}=\widetilde{\mathbf{N}}'} P^{s}_{\widetilde{\mathbf{N}}} = \left[\frac{N!}{\prod_{a=1}^{n'}\widetilde{N}'_a!}\prod_{b=1}^{n'}\left(\frac{N_b'^{s}}{N}\right)^{\widetilde{N}'_b}\right]\sum_{\widetilde{\mathbf{N}}}\prod_{c=1}^{n'}\left(\frac{\widetilde{N}'_c!}{N_c'^{s\,\widetilde{N}'_c}}\prod_{i\in S_c}\frac{N_i^{s\,\widetilde{N}_i}}{\widetilde{N}_i!}\right)\delta^{\widetilde{N}'_c}_{\sum_{k\in S_c}\widetilde{N}_k}, \qquad (3.2)$$

with $\sum_{i=1}^{n}\widetilde{N}_i = N$, where $\sum_{\widetilde{\mathbf{N}}}$ is as defined in (2.2) and $\delta_X^{X'}$ is the same as that in (2.5). With the same argument in the text following (2.6), (3.2) can be reexpressed as,

$$\sum_{\mathbf{U}\widetilde{\mathbf{N}}=\widetilde{\mathbf{N}}'} P^{s}_{\widetilde{\mathbf{N}}} = \left[\frac{N!}{\prod_{a=1}^{n'}\widetilde{N}'_a!}\prod_{b=1}^{n'}\left(\frac{N_b'^{s}}{N}\right)^{\widetilde{N}'_b}\right]\prod_{c=1}^{n'}\frac{1}{N_c'^{s\,\widetilde{N}'_c}}\underbrace{\sum_{\{\widetilde{N}_j\mid j\in S_c\}}\widetilde{N}'_c!\left(\prod_{i\in S_c}\frac{N_i^{s\,\widetilde{N}_i}}{\widetilde{N}_i!}\right)\delta^{\widetilde{N}'_c}_{\sum_{k\in S_c}\widetilde{N}_k}}_{\equiv(\#)}. \qquad (3.3)$$

Due to the multinomial relation $\sum_{n_1,n_2,\ldots} m!\prod_i x_i^{n_i}/n_i! = \left(\sum_i x_i\right)^m$ with $\sum_i n_i = m$, the sum (#) in (3.3) can be simplified as

$$\sum_{\{\widetilde{N}_j\mid j\in S_c,\ \sum_{k\in S_c}\widetilde{N}_k=\widetilde{N}'_c\}}\widetilde{N}'_c!\prod_{i\in S_c}\frac{N_i^{s\,\widetilde{N}_i}}{\widetilde{N}_i!} = \left(\sum_{i\in S_c}N_i^s\right)^{\sum_{j\in S_c}\widetilde{N}_j} = N_c'^{s\,\widetilde{N}'_c}, \qquad (3.4)$$

where the TE condition, $N_c'^{s} = \sum_{i\in S_c}N_i^s$, has been used in the last equality in (3.4). Inserting

(3.4) into (3.3), the product $\prod_{c=1}^{n'} \dots$ in (3.3) is reduced to one. Thus (3.3) becomes

$$\sum_{\mathbf{U}\tilde{\mathbf{N}}=\tilde{\mathbf{N}}'} P_{\tilde{\mathbf{N}}}^{S} = \frac{N!}{\prod_{a=1}^{n'} \tilde{N}_a'!} \prod_{b=1}^{n'} \left(\frac{N_b'^{S}}{N}\right)^{\tilde{N}_b'} = P'^{S}_{\tilde{\mathbf{N}}'}, \tag{3.5}$$

which is the steady-state distribution of the CME of a lumped system.

To see the reverse direction that $\mathbf{P}'^{S} = \hat{\mathbf{U}}\mathbf{P}^{S}$ implies $\mathbf{N}'^{S} = \mathbf{U}\mathbf{N}^{S}$, one needs only to replace $P_{\tilde{\mathbf{N}}}$ in (2.11) by $P_{\tilde{\mathbf{N}}}^{S}$ here and follow the same argument in (2.11). ■

**S4. The indistinguishable $\boldsymbol{\Gamma}$ of intrinsic noises**

The $\boldsymbol{\Gamma}$ of network $A$ in the main text is

$$\boldsymbol{\Gamma} \equiv \left[\sum_{k=1}^{n} (k_{ki}N_k + k_{ik}N_i)\right]\delta_{ij} - k_{ji}N_j - k_{ij}N_i. \tag{4.1}$$

<u>**Claim**</u>: If $A$ can be exactly lumped into $A'$ by $\mathbf{U}$, $\boldsymbol{\Gamma}$ of $A$ and $\boldsymbol{\Gamma}'$ of $A'$ follow the relation

$$\boldsymbol{\Gamma}' = \mathbf{U}\boldsymbol{\Gamma}\mathbf{U}^{T}. \tag{4.2}$$

<u>Proof</u>:
Replacing the index $j$ in (1) by $k$ and multiplying that equation with $\delta_{ij}$, the RE of $A$ becomes a matrix equation whose entries indexed by $(i,j)$ obey

$$\frac{dN_i}{dt}\delta_{ij} = \left[\sum_{k=1}^{n} (k_{ki}N_k - k_{ik}N_i)\delta_{ij}\right]$$

$$= \left[k_{ji}N_j - \sum_{k=1}^{n} k_{ik}N_i\delta_{ij}\right] + \left[-k_{ji}N_j + \sum_{k=1}^{n} k_{ki}N_k\delta_{ij}\right]. \tag{4.3}$$

It can be expressed as

$$\frac{d\mathbf{D_N}}{dt} = \boldsymbol{\Pi} + \boldsymbol{\Pi}^{(\mathrm{C})^{T}}, \tag{4.4}$$

with the diagonal matrix $[\mathbf{D_N}]_{ij} = N_i\delta_{ij}$, $\boldsymbol{\Pi} \equiv \mathbf{M}\mathbf{D_N}$, and the last term in (4.3) has been denoted by $\boldsymbol{\Pi}^{(\mathrm{C})^{T}}$. In analogy, the RE of $A'$ has the matrix equation,

$$\frac{d\mathbf{D_{N'}}}{dt} = \boldsymbol{\Pi}' + \boldsymbol{\Pi}'^{(\mathrm{C})^{T}}, \tag{4.5}$$

with $\boldsymbol{\Pi}' \equiv \mathbf{M}'\mathbf{D_{N'}}$. Operating $\mathbf{U}$ and $\mathbf{U}^{T}$ on the left and right hand sides of (4.4) leads to

$$\frac{d\mathbf{U}\mathbf{D_N}\mathbf{U}^{T}}{dt} = \mathbf{U}\boldsymbol{\Pi}\mathbf{U}^{T} + \mathbf{U}\boldsymbol{\Pi}^{(\mathrm{C})^{T}}\mathbf{U}^{T}. \tag{4.6}$$

Under the KE condition, one can readily see

$$\mathbf{U}\mathbf{D}_\mathbf{N}\mathbf{U}^\mathbf{T} = \mathbf{D}_{\mathbf{N}'}, \tag{4.7}$$

and (4.6) and (4.5) are the same rate equations. Inserting

$$\mathbf{U\Pi U}^T = \mathbf{UMD}_\mathbf{N}\mathbf{U}^T = \mathbf{M}'\mathbf{UD}_\mathbf{N}\mathbf{U}^T = \mathbf{M}'\mathbf{D}_{\mathbf{N}'} = \mathbf{\Pi}', \tag{4.8}$$

implied from (4.7) into (4.6) and comparing (4.6) with (4.5), one obtains

$$\mathbf{\Pi}'^{(\mathrm{C})} = \mathbf{U}\mathbf{\Pi}^{(\mathrm{C})}\mathbf{U}^T. \tag{4.9}$$

In terms of the notations in (4.4), the $\mathbf{\Gamma}$ in (4.1) can be expressed as

$$\Gamma_{ij} = -\left[k_{ji}N_j - \sum_{k=1}^{n} k_{ik}N_i\delta_{ij}\right] + \left[-k_{ij}N_i + \sum_{k=1}^{n} k_{ki}N_k\delta_{ij}\right],$$

$$\mathbf{\Gamma} \equiv -\mathbf{\Pi} + \mathbf{\Pi}^{(\mathrm{C})}. \tag{4.10}$$

Operating $\mathbf{U}$ and $\mathbf{U}^T$ onto (4.10) and using (4.8) and (4.9), it yields

$$\begin{aligned}\mathbf{U\Gamma U}^\mathbf{T} &= -\mathbf{U\Pi U}^T + \mathbf{U}\mathbf{\Pi}^{(\mathrm{C})}\mathbf{U}^T \\ &= -\mathbf{\Pi}' + \mathbf{\Pi}'^{(\mathrm{C})} = \mathbf{\Gamma}',\end{aligned} \tag{4.11}$$

which is the claim in (4.2). ■
